# Supplementary material for: Efficient displacement convex optimization with particle gradient descent
Source: arXiv:2302.04753 source file (2023-02-09)
Supplement: Supplementary file 1 [file appendix.tex]

\section{Displacement convexity}
\subsection{Proof of Proposition~\ref{proposition:non-convex}}
Suppose that $w_1^*, \dots, w_n^*$ is the unique minimizer of $F$ such that $w_1^* \neq w_2^*$. Let $\sigma$ is a non monotone permutation of $\{1,\dots, n\}$. Interpolating the parameters $\{w_i^*\}$ with the permuted $\{w_{\sigma(i)}^*\}$ concludes $F$ is not convex since
\begin{align*}
   F\left(\frac{1}{n}\sum_{i=1}^n \delta_{(1-t)w_i^* + t w_{\sigma(i)}^* }\right) > t F\left(\frac{1}{n}\sum_{i=1}^n \delta_{w_i^*}\right) + (1-t) F\left(\frac{1}{n}\sum_{i=1}^n \delta_{w_{\sigma(i)^*}}\right)
\end{align*}
holds for the unique minimizer $w_1^*,\dots, w_n^{*}$. Thus, $F$ is not convex. 

\subsection{Proof of Proposition~\ref{prop:Lipschitz}}
 
The range of $\Phi$ lies in a Hilbert space with a norm induced by an inner product. Thus, 
\begin{align*}
    \left\| \int \Phi d\mu - \int \Phi d\nu  \right\|^2 & =  \left\langle \int \Phi d\mu - \int \Phi d\nu, \int \Phi d\mu - \int \Phi d\nu \right\rangle \\ 
    & =  \left\langle \int \Phi d\mu,  \int \Phi d\mu \right\rangle - 2  \left\langle \int \Phi d\mu,  \int \Phi d\nu \right\rangle + \left\langle \int \Phi d\nu,  \int \Phi d\nu \right\rangle \\ 
    & = \left( \text{MMD}_K(\mu,\nu)\right)^2.
\end{align*}
 The above result together with the Lipschitz property of $R$ conclude the proof.

\subsection{Example ~\ref{lemma:weakconvex_w2}}
\begin{align*}
\text{Define:} \quad \quad &
   \sigma^*= \arg \underbrace{\min_{\sigma} \sum_{i=1}^n \| w_i - v_{\sigma(i)}\|^2}_{=W_2^2(\mu,\nu)}. \\
   \text{Define:} \quad \quad & \mu_t = \frac{1}{n} \sum_{i=1}^n \delta_{(1-t)w_i + t v_{\sigma^*(i)}}.
\end{align*}
According to definition of $W_2$, we have
\begin{align*}
    W_2(\mu_t,\nu) \leq \sum_{i=1}^n \| (1-t) w_i + t v_{\sigma^*(i)} - v_{\sigma^*(i)}\|^2 = (1-t) W_2^2(\mu,\nu) + \underbrace{t W_2^2(\nu,\nu)}_{=0}.
\end{align*}

\subsection{Example~\ref{example:tensor}}

\begin{align*}
   \text{Define:} \quad \quad  &\sigma = \arg\min_{\sigma'} \sum_{i} \left\| w_{i}- v_{\sigma'(i)} \right\|^2. \\
   \text{Define:} \quad \quad &
     g(t) = G\left(\underbrace{(1-t) w_1 + t v_{\sigma(1)}}_{w_1(t)},\dots, (1-t) w_n + t v_{\sigma(n)}\right).
\end{align*}

To prove $G$ is star displacement convex, we need to prove that $
     - g'(0) \geq (G -G^*)$ holds.
To validate this inequality, we take the derivative of $g$ with respect to $t$: 
% \begin{multline}
%     \frac{1}{4}g'(t) =  -\sum_{i} \left( \frac{\langle v_i, x_t \rangle^3 \langle v_i, (v_j-x) \rangle}{\| x_t \|^4} + \frac{\langle v_i,(1-t)x\rangle^4(1-x^\top v_j)}{\|x_t\|^4}\right)  
% \end{multline}
\begin{align*}
       \frac{1}{3}g'(t) =  -\sum_{j} \sum_{i} \left( \frac{\langle v_i, w_j(t) \rangle^2 \langle v_i, (v_{\sigma(j)}-w_j(t)) \rangle}{\| w_j(t) \|^3} + \frac{\langle v_i,w_j(t)\rangle^3 \langle w_j(t),w_j- v_{\sigma(j)}\rangle }{\|w_j(t)\|^3}\right). 
\end{align*}
For $w_1,\dots, w_n \in \mathcal{S}_{d-1}$, we get
\begin{align}
     \frac{1}{3}g'(0) = \sum_{j} \langle w_j,v_{\sigma(j)}\rangle \left( \sum_{i} \langle v_i, w_j \rangle^3 - \langle w_j, v_{\sigma(j)} \rangle \right),
 \end{align}
 where we used the orthogonality of $v_1,\dots, v_n$.
 Since $\sigma$ is an optimal permutation, we have 
\begin{align}
     n \sum_{j} \langle w_j , v_{\sigma(j)} \rangle^2 \geq \sum_{i} \sum_{j} \langle w_i, v_{j} \rangle^2 =  n,
\end{align}
where we use the orthogonality of $v_1,\dots, v_n$ to get the last equality. 
Therefore, 
\begin{align}
     -\frac{1}{3}g'(0) & \geq 1 - \sum_{i,j=1}^n \langle v_i, w_j \rangle^3 = G - G^*
\end{align}

\subsection{Properties of $\lambda$-convex functions}
Let  $T$ denote the optimal transport from $\mu$ to $\nu$ which achieves  
\begin{align}
 W_2^2(\mu,\nu) =\sum_{i=1}^n \| w_i - T(w_i)\|^2_2
\end{align}

 Let $g(t) = F(\mu_t)$ where $\mu_t$ is obtained by the displacement interpolation of $\mu$ and $\nu$. Taking the derivative of $g$ with respect to $t$ leads to the following important inequality \cite{santambrogio2017euclidean}:
\begin{align} \label{eq:gradient_bound}
    \underbrace{\sum_{i} \langle w_i-T(w_i), \partial_{w_i} F(\mu)\rangle}_{g'(0)} &\geq F(\mu) - F(\nu) +\frac{\lambda}{2} W_2^2(\mu,\nu)
\end{align}

\subsection{Properties of smooth and displacement convex functions}
 The next Theorem establishes properties of smooth and displacement convex functions.
\begin{theorem} \label{thm:smoothness_consequences}
An $\ell$-smooth $F$ and $(\lambda\geq 0)$-displacement convex function obeys 

    \begin{equation} \tag{i} \sum_{i} \| \partial_{w_i} F(\mu) - \partial_{T(w_i)} F(\nu) \| \leq \ell^2 W_2^2(\mu,\nu)
    \end{equation}
    \begin{equation} \tag{ii}\| \partial_{w_i} F(\mu) - \partial_{w_j} F(\mu) \| \leq \ell \| w_i - w_j\| 
    \end{equation}
    \begin{equation} \tag{iii} F(\nu) \geq  F(\mu) + \sum_{i} \langle \partial_{w_i} F(\mu), T(w_i) - w_i  \rangle +\frac{1}{2\ell} \sum_{i} \| \partial_{T(w_i)}F(\nu) - \partial_{w_i} F(\mu)\|^2
    \end{equation}
    \begin{equation} \tag{iv} \label{eq:iv} \sum_{i} \langle \partial_{T(w_i)} F(\nu) - \partial_{w_i} F(\nu), T(w_i) - w_i  \rangle \geq \frac{1}{\ell} \sum_{i} \| \partial_{T(w_i)}F(\nu) - \partial_{w_i} F(\mu)\|^2 
    \end{equation}
     \begin{multline} \quad \tag{v}
        \sum_{i}\langle \partial_{w_i} F(\mu)- \partial_{T(w_i)} F(\nu), w_i - T(w_i) \rangle \geq \frac{\lambda \ell}{\ell+\lambda} \sum_i \| w_i - T(w_i) \|^2 + \frac{1}{\lambda + \ell}\| \partial_{w_i} F(\mu) - \partial_{w_i} F(\nu)\|^2 \label{eq:v}
    \end{multline} 

\end{theorem}
\begin{proof}
\textbf{(i)}
Since the smoothness holds for all permutation of particles, we get 
\begin{align}
      \sum_{i=1}^n \| \partial_{w_i} F(\mu) - \partial_{T(w_i)} F(\nu) \|^2 
     & = \| \partial F(w) - \partial F(v)\|^2\\ 
     & \leq \ell^2 \|w - v \|^2 = \ell^2 W_2^2(\mu,\nu),
\end{align}
where use a permutation of particles to get the the last equality.\\
\textbf{(ii)}
Suppose that $v$ is obtained by swapping $w_i$ and $w_j$ for $i\neq j$ in $w=(w_1,\dots, w_n)$. Then, the smoothness implies 
\begin{align}
     \| \partial_{w_i} F(w) - \partial_{w_j} F(v) \| \leq \ell \| w_i - w_j\|  \label{eq:smoothness_consequence}
\end{align}
% \subsection*{Part III} Let $h_t(w) = (1-t) w + t T(w)$; then,
% \begin{align}
%     F(\nu) - F(\mu) - \int \langle \partial_w F(\mu), T(w) - w  \rangle d\mu(w) & \leq \int_{0}^1  \int \langle \partial_{h_t(w)} F(\mu_t)- \partial_w F(\mu), T(w) - w  \rangle d\mu(w) dt \nonumber \\ 
%     & \leq W_2(\mu,\nu) \max_{t\in [0,1]} \sqrt{\frac{1}{n}\sum_{i=1}^n \|\partial_{h_t(w_i)} F(\mu_t)- \partial_{w_i} F(\mu) \|^2  } \\
%     & \leq \ell W_2(\mu,\nu) \max_{t \in [0,1]} W_2(\mu_t,\nu) \\
%     & \leq \ell W_2^2(\mu,\nu)
% \end{align}
\textbf{(iii)}
Akin to the proof of
Theorem 2.1.5 in \cite{nesterov1999global}, we define
\begin{align*}
   Q(\nu) = F(\nu) - \sum_{i} \langle T(w_i), \partial_{w_i} F(\mu) \rangle
\end{align*}
Displacement convexity, more precisely  Eq.~\eqref{eq:gradient_bound}, ensures that $\mu$ is the minimizer of the above functional since 
\begin{align}
 F(\nu) - F(\mu) - \sum_{i} \langle T(w_i)-w_i, \partial_{w_i} F(\mu)\rangle \geq 0
\end{align}
$\ell$-smoothness ensures \cite{nesterov1999global} 
\begin{align}
    Q(\mu) & \leq Q\left( \frac{1}{n} \sum_{i=1}^n \delta_{v_i - \frac{1}{\ell} \partial_{v_i} Q(\nu)}\right) \\ 
    &\leq Q(\nu) - \frac{1}{2\ell} \underbrace{\sum_{i=1}^n \| \partial_{v_i} Q(\nu)\|^2}_{= \sum_{i} \|\partial_{T(w_i)} F(\nu) - \partial_{w_i}  F(\mu) \|^2 }
\end{align}

\end{proof}
We will repeatedly use the above inequalities in future analysis. 

\noindent
\textbf{(iv)} Inequality (iii) ensures 
\begin{align}
    F(\nu) & \geq  F(\mu) + \sum_{i} \langle \partial_{w_i} F(\mu), T(w_i) - w_i  \rangle +\frac{1}{2\ell} \sum_{i} \| \partial_{T(w_i)}F(\nu) - \partial_{w_i} F(\mu)\|^2 \\
     F(\mu) & \geq  F(\nu) + \sum_{i} \langle \partial_{T(w_i)} F(\nu), w_i - T(w_i)  \rangle +\frac{1}{2\ell} \sum_{i} \| \partial_{T(w_i)}F(\nu) - \partial_{w_i} F(\mu)\|^2
\end{align}

Summing up the above two inequalities concludes (iv). 

\noindent
\textbf{(v)} The proof is similar to the proof of Theorem 2.1.11 in \cite{nesterov1999global}. Recall $T$ is the optimal transport map from $\mu$ to $\nu$ and $\mu_t$ is the displacement interpolation between $\mu$ and $\nu$. First, we define function $\phi(\mu) = F(\mu) - \frac{\lambda}{2} \sum_{i=1}^n \| w_i \|^2$. We prove $\phi$ is $0$-displacement convex.  
\begin{align}
    \phi(\mu_t) & \leq (1-t) F(\mu) + t F(\nu) - \left(\frac{(1-t) t \lambda }{2}\right)W_2^2(\mu,\nu) \\ 
    \phi(\mu) & = F(\mu) - \frac{\lambda}{2} \sum_{i=1}^n \| w_i\|^2 \\ 
    \phi(\nu) & = F(\nu) - \frac{\lambda}{2} \sum_{i=1}^n \| T(w_i)\|^2
\end{align}
Putting the above three equations together yields
\begin{multline}
    (1-t) \phi(\mu) + t \phi(\nu) - \phi(\mu_t) \geq \left(\frac{\lambda t (1-t)}{2}\right) \sum_{i} \| w_i - T(w_i)\|^2 \\ 
    - \frac{\lambda(1-t)}{2} \sum_{i}\|w_i\|^2 - \frac{\lambda}{2} \sum_{i} \|T(w_i)\|^2 \\ 
    + \frac{\lambda}{2} \sum_{i} \| (1-t) w_i + t T(w_i)\|^2 
\end{multline}
Expanding the last term concludes $\phi$ is $0$-displacement convex. Thus, we can use (\ref{eq:iv}) to get
\begin{align}
   \sum_{i} \langle \partial_{w_i} \phi(\mu) - \partial_{T(w_i)} \phi(\nu), w_i - T(w_i) \rangle \geq \frac{1}{\ell-\lambda} \sum_{i} \| \partial_{w_i} \phi(\mu) - \partial_{T(w_i)} \phi(\nu) \|^2
\end{align}
A rearrangement of the terms concludes (v).

\section{Smooth displacement convex optimization}

\subsection{Proof of Theorem~\ref{thm:smooth}.a}
\subsection*{Contraction}

We first prove that the particles contract in $W_2$.
\begin{lemma}[Contraction] \label{lemma:contraction}
Suppose that $\mu_{k}$ is obtained by particle gradient descent starting from $n$-sparse measures with distinct particles. If $F$ is $\lambda$-displacement convex and $\ell$-smooth, then  
\begin{align}
    W_2^2(\mu_{(k+1)},\widehat{\mu}) \leq \left(1-\left(\frac{2 \lambda \ell \gamma}{\ell+\lambda}\right)\right) W_2^2(\mu_{k},\widehat{\mu})
\end{align}
holds for $\gamma \leq 2/(\ell+L)$.
\end{lemma}
\begin{proof}
In order to leverage displacement convexity, we need to ensure the optimal transport map exists from $\mu_{(k)}$ to $\widehat{\mu}$ for all $k$. 
 The next Lemma proves that  $\mu_k$ has distinct particles assuming $\mu_0$ has distinct particles, hence the optimal transport map exists under weak conditions on $\mu_0$.
 \begin{lemma} \label{lemma:smooth_dist} For $\ell$-smooth $F$ and $\gamma<1/\ell$, $w_i^{(k+1)} = w_j^{(k+1)}$ hold only if $w_i^{(k)} = w_j^{(k)}$.
\end{lemma}
 Therefore, the optimal transport from $\mu:= \mu_k$ to $\widehat{\mu}$  is well defined and denoted by $T$. We leverage this transports to couple  $\mu_+ := \mu_{k+1}$ with $\widehat{\mu}$. The optimality of the transport implies that 
\begin{align}
    \sum_{i} \| w_i - T(w_i) \|^2 d\mu(w) = W_2^2(\mu,\widehat{\mu})
\end{align}
Using the recurrence of gradient descent, we get 
\begin{align}
    W_2^2 \left( \mu_{+} , \widehat{\mu} \right)  \leq  \sum_{i} \left(  \| w_i - T(w_i) \|^2  + 2 \gamma \langle T(w_i) - w_i, \partial_{w_i} F(\mu)  \rangle\right) +  
     \gamma^2 \sum_{i} \| \partial_{w_i} F(\mu)  - \underbrace{\partial_{T(w_i)} F(\widehat{\mu})}_{=0} \|^2.
\end{align}
% According to Theorem~\ref{thm:smoothness_consequences}.\ref{eq:v}. we have
% \begin{align}
%     \sum_{i} \| \partial_{w_i} F(\mu)  - \partial_{T(w_i)} F(\widehat{\mu}) \|^2 \leq \ell^2 W_2^2(\mu,\widehat{\mu}).
% \end{align}
According to Theorem~\ref{thm:smoothness_consequences}.\ref{eq:v}. we have
\begin{align*}
    \sum_{i} 
    \left(\langle w_i - T(w_i), \partial_{w_i} F(\mu) \rangle\right)  \geq \frac{\lambda \ell}{\ell+\lambda} W_2^2(\mu,\widehat{\mu}) + \frac{1}{\ell+\lambda} \sum_{i} \| \partial_{w_i} F(\mu)- \partial_{T(w_i)} F(\widehat{\mu}) \|^2
\end{align*}
Combining the last two inequalities, we get 
\begin{align*}
W_2^2(\mu_{+},\widehat{\mu}) \leq W_2^2(\mu,\widehat{\mu}) -  \left(\frac{2 \lambda \ell \gamma}{\ell+\lambda}\right)W_2^2(\mu,\widehat{\mu}) + \left(\gamma^2 -\frac{2\gamma}{\ell+\lambda}\right)\sum_{i} \| \partial_{w_i} F(\mu)  - \underbrace{\partial_{T(w_i)} F(\widehat{\mu})}_{=0} \|^2
\end{align*}
For $\gamma \leq 2/(\ell+\lambda) $, we get 
\begin{align}
      W_2^2(\mu_{+},\widehat{\mu}) \leq  \left(1-\left(\frac{2 \lambda \ell \gamma}{\ell+\lambda}\right)\right) W_2^2(\mu,\widehat{\mu}).
\end{align}

\end{proof}
\subsection*{Convergence proof}

A straight forward applications of Cauchy-Schwarz for Eq.\ref{eq:gradient_bound} yields
\begin{align}
     W_2(\mu,\widehat{\mu}) \sqrt{ \sum_{i} \| \partial_{w_i} F(\mu)\|^2 } \geq F(\mu) - F(\widehat{\mu})
\end{align}
holds for all $\mu$ with $n$ particles.
Invoking Theorem~\ref{thm:smoothness_consequences}.I, we get 
\begin{align}
    \sum_{i} \| \partial_{w_i} F(\mu)\|^2  \leq \ell^2 W_2^2(\mu,\widehat{\mu})
\end{align}
Combining the last two inequalities, we get
\begin{align}
    F(\mu) - F(\widehat{\mu}) \leq \ell W_2^2(\mu,\widehat{\mu})
\end{align}
Combining the above inequality with the contraction established in the last lemma, we get
\begin{align}
     |F(\mu_{k+1}) - F(\widehat{\mu})| \leq \ell \left(1- \frac{2 \lambda \ell \gamma}{\ell+\lambda}\right)^k  W_2^2(\mu_0,\widehat{\mu}) 
\end{align}
\subsection{Proof of Theorem~\ref{thm:smooth}.c.} 
It is known that gradient descent decreases smooth functions in each iteration as long as $\gamma \leq 1/\ell$ (see Theorem 2.1.13 of \cite{nesterov1999global}): 
\begin{align} \label{eq:f_decrease_smooth}
 F(\mu_{k+1}) \leq F(\mu_k) - \gamma \left(1- \ell \gamma/2 \right) \sum_{i} \| \partial_{w_i} F(\mu_k)\|^2  
\end{align}
star displacement convexity ensures
 \begin{align}
       \sum_{i} \langle w_i-T(w_i), \partial_{w_i} F(\mu) \rangle  \geq  F(\mu_k) - F(\widehat{\mu}).
 \end{align}
 A straightforward application of Cauchy-Schwarz yields 
 \begin{align}
    \sum_i \langle w_i - T(w_i), \partial_{w_i} F(\mu) \rangle &\leq \sum_{i} \| w_i - T(w_i)\| \| \partial_{w_i} F(\mu)\| \\ 
     & \leq W_2(\mu_k,\widehat{\mu}) \sqrt{\sum_{i} \| \partial_{w_i} F(\mu)\|^2 }
 \end{align}
where the last inequality holds since $W_2^2(\mu_k,\widehat{\mu})$ is decreasing for $\gamma<1/\ell$.
Combining the last two inequalities, we get 
\begin{align}
    \sum_i \| \partial_{w_i} F(\mu)\|^2 \geq \frac{\left( F(\mu_k) - F(\widehat{\mu})\right)^2}{W_2^2(\mu_k,\widehat{\mu})} 
\end{align}
We introduce the compact notion $\Delta_k = F(\mu_k) - F(\widehat{\mu})$. Plugging the last inequality into Eq.~\ref{eq:f_decrease_smooth} obtains 
\begin{align}
    \Delta_{k+1} & \leq \Delta_k - \underbrace{\left(\frac{\gamma}{W_2^2(\mu_k,\widehat{\mu})}\right)}_{\geq \gamma/r^2}(1-\ell\gamma/2) \Delta_k^2 
\end{align}
According to Theorem 2.1.13 of \cite{nesterov1999global}, the above inequality concludes the proof.
\begin{align}
     \frac{1}{\Delta_{k+1}} \geq \frac{1}{\Delta_k (1-c\Delta_k)}
\end{align}
\subsection{Proof of Theorem~\ref{thm:smooth}.b}
%The proof is similar to Theorem 2.1.13 of \cite{nesterov1999global}. 
Suppose that $T$ is the optimal transport map from $\mu_k$ to $\widehat{\mu}$. Using $\ell$-smoothness, we have
\begin{align}
    W_2^2  (\mu_{k+1}, \widehat{\mu} )  \leq \sum_{i}  \| T(w_i) - w_i \|^2 +  2 \gamma  \langle T(w_i) - w_i, \partial_{w_i} F(\mu_k) \rangle  + 
     \gamma^2 \| \partial_{w_i} F(\mu_k)  \|^2
\end{align}
 Replacing $\nu = \widehat{\mu}$ and $\mu= \mu_k$ in Theorem~\ref{thm:smoothness_consequences}.III yields
\begin{align}
  \sum_i \langle w_i-T(w_i),\partial_{w_i} F(\mu) \rangle \geq \frac{1}{2\ell} \sum_{i} \| \partial_{w_i} F(\mu) \|^2 
\end{align}
Incorporating the above inequality into the established bound for $W_2$ leads to 
\begin{align}
    W_2^2(\mu_{k+1},\widehat{\mu}) \leq W_2^2(\mu_k,\widehat{\mu}) + (\gamma^2-\gamma/\ell) \sum_i \| \partial_{w_i} F(\mu_k)\|^2.
\end{align}
Thus, $W_2(\mu_k,\widehat{\mu})$ is non-increasing in $k$ for $\gamma\leq 1/\ell$. Since a $0$-displacement convex function is also weak displacement convex, invoking part c. of Theorem~\ref{thm:smooth} with $r^2 = W_2^2(\mu_0,\widehat{\mu})$ concludes the proof.

% \subsection{Proof of Proposition~\ref{lemma:saddles}} 
% The optimality condition concludes that $\partial_{w_i} F(\frac{1}{n} \sum_{i=1}^{n-1} \delta_{\widehat{w}_i} + \frac{1}{n}\delta_{\widehat{w}_{n-1}}) = 0$ for all $i$. However, the uniqueness $(w_1^*,\dots, w^*_n)$ and $w_i^* \neq w_j^*$ is not the minimizer of $F$.  
\subsection{Proof of Lemma~\ref{lemma:smooth_dist}}

The proof is similar to the analysis of smooth programs in \cite{lee2016gradient}. According to the definition, $w_{i}^{(k+1)}= w_j^{(k+1)}$ if  
\begin{align}
    w_i^{(k)} - \gamma \partial_{w_i} F(\mu_k) =  w_j^{(k)} - \gamma \partial_{w_i} F(\mu_k) 
\end{align}
A rearrangement of terms together with Theorem~\ref{thm:smoothness_consequences}.II concludes the proof: 
\begin{align} 
\| w_i^{(k)} - w_j^{(k)}\| = \gamma  \|\partial_{w_i} F(\mu_k)- \partial_{w_j} F(\mu_k) \| \leq \gamma \ell \| w_i^{(k)}- w_j^{(k)} \| < \| w_i^{(k)} - w_j^{(k)}\|.
\end{align}
\section{Lipschitz displacement convex optimization}
% \subsection{Proof of Lemma~\ref{lemma:collision}}
% Consider minimization of $\min E(\mu,\nu)$ defined in Eq.~\ref{eq:mmd}. For all $\mu_{0} = \frac{1}{n} \sum_{i=1}^n \delta_{w_i}$ such that $w_1^{(0)} \geq w_2^{(0)} \geq \dots \geq w_n^{(0)}$ and $| w_1^{(0)} - w_2^{(0)}| \leq \gamma(1/n-1/n^2)$, there exits a probability measure $\nu$ such that $w_1^{(k)} = w_2^{(k)}$ for all $k\geq 1$. 
% Without loss of generality, we assume that $w_1^{(0)}>w_2^{(0)}$ holds. According to \cite{hadi22}, we can alternatively write the gradient of $F$ as
% \begin{align}
%      \partial_{w_i} F(\mu) =  \frac{2}{n} \left( \int^{w_i} \nu d(w) - \int^{w_i} \mu d(w)  \right)
% \end{align}
% Thus, 
% \begin{align}
%     w^{(1)}_1 - w^{(1)}_2 = \frac{2\gamma}{n} \left( \int_{w_{2}^{(0)}}^{w_{1}^{(0)}} d \nu (w) - \frac{1}{n} \right)
% \end{align}
% We define $\nu$ in interval $[w_2^{(0)},w_1^{(0)}]$ such the equality is met. If $w_1^{(1)} = w_2^{(1)}$, then these particle remain equal during all descent steps of particle gradient descent. 

\subsection{Proof of Theorem~\ref{thm:nonsmooth}.a}
The proof is inspired by the convergence analysis of gradient descent for non-smooth convex functions (Theorem 3.9 of \cite{bubeck2015convex}). The injection with noise ensures that the particles remain distinct with probability one, hence the optimal transport from $\mu_k$ to $\widehat{\mu}$ denoted by $T$ exists with probability one. Leveraging the optimal transport $T$ and inequality~\ref{eq:gradient_bound} obtained by $\lambda$-diplacement convexity, we get
\begin{multline}
   \E\left[ W_2^2 \left( \mu_{k+1} , \widehat{\mu} \right) \right] \leq \E \left[ \sum_{i}  \| T(w_i) - w_i \|^2  + \gamma_k\underbrace{2 \sum_{i}   \langle T(w_i) - w_i, \partial_{w_i} F'(\mu_k) \rangle}_{\leq -\lambda W_2^2(\mu_k,\widehat{\mu}) + 2F(\widehat{\mu})-2F(\mu_k)) } \right]    \\ + 
     \gamma^2_k \underbrace{\sum_{i} \E  \| \partial_{w_i} F(\mu_k) \|^2 }_{\leq L^2} 
     +  \frac{\gamma^2_k}{n}\sum_{i=1}^n \E \left[ \| \xi_i^{(k)}\|^2 \right]
\end{multline} 
A rearrangement of terms yields 
\begin{multline}
   k \E \left[  F(\mu_k) - F(\widehat{\mu}) \right]  \\ \leq \lambda k(k-1) \E \left[ W_2^2(\mu_k,\widehat{\mu}) \right] - \lambda k(k+1) \E \left[ W_2^2(\mu_{k+1},\widehat{\mu})\right]+\frac{(L^2+1)}{\lambda}
\end{multline}
Summing over $k=1,\dots,m$ concludes the proof as 
\begin{align}
   \left(\frac{m(m+1)}{2}\right) \min_{k\leq m} \left( \E \left[ F(\mu_k) - F(\widehat{\mu}) \right] \right) \leq \sum_{k=1}^m k\left( \E \left[ F(\mu_k) - F(\widehat{\mu})\right] \right) \leq  \frac{m(L^2+1)}{\lambda}.
\end{align}

\subsection{Proof of Theorem~\ref{thm:nonsmooth}.b} \noindent The proof is inspired by convex analysis for non-smooth functions (Theorem 3.2.2 of \cite{nesterov1999global}). Suppose $\widehat{\mu}$ the minimzier of particle program and let $T$ denotes the optimal mapping from $\mu_{k}$ to $\widehat{\mu}$. The injection with noise ensure that particles of $\mu_k$ are distinct, hence $T$ does exists.  
\begin{multline}
    \E \left[ W_2^2 \left( \mu_{k+1} , \mu_* \right) \right]  \leq \E \left[ \sum_{i} \left(  \| T(w_i) - w_i \|^2  + 2 \gamma \langle T(w_i) - w_i, \partial_{w_i} F(\mu_k) \rangle \right)  \right] \\ + 
     \gamma^2 \underbrace{ \sum_{i} \E \| \partial_{w_i} F(\mu)  \|^2 }_{\leq L^2} 
     +  \frac{\gamma^2}{n}\sum_{i=1}^n \E \| \xi_i^{(k)}\|^2 
\end{multline} 
Using Eq.~\eqref{eq:gradient_bound}, we conclude that 
\begin{align}
     -\int \langle T(w) - w, \partial_w F(\mu)\rangle d \mu_k(w) \geq \underbrace{F(\mu_k) - F(\widehat{\mu})}_{\Delta_k} \geq 0
\end{align}
Therefore, 
\begin{align} 
 \E \left[  W_2^2 \left( \mu_{k+1} , \widehat{\mu} \right) \right] \leq  \E \left[ W_2^2 \left( \mu_{k} , \widehat{\mu}\right) \right] - 2\gamma \E \left[ \Delta_k \right] + \gamma^2 (L^2+1) 
\end{align}
Summing over $k$ concludes the proof
\begin{align}
  (m\gamma) \min_{k \in \{1, \dots, m\}} \E \left[ \Delta_k \right] \leq   \sum_{k=1}^m \gamma \E \left[ \Delta_k \right] \leq W_2^2(\mu_0,\widehat{\mu}) + m \gamma^2 (L^2+1)
\end{align}

\section{Approximation error}
\subsection{Proof of Lemma~\ref{lemma:approx_convex}}
The proof is based on the convergence of Frank-Wolf algorithm. This proof technique is previously used for specific functions in neural networks~\cite{bach2017breaking}.  Since this algorithm uses a (infinite-dimensional) non-convex optimization in each step, it is not implementable. Yet, we can use its convergence properties to bound the approximation error. 
To introduce the algorithm, we first need to formulate the optimization over a compact domain in Banach space. We optimize $F$ over $L^2$ Hilbert spaces of functions.  Let $D$ is the set of probability measures over a compact set, which is a subset of $L^2$. Frank-Wolfe method optimizes $F$ through the following iterations \cite{jaggi2013revisiting}
\begin{align}
   \mu^{(k+1)} = (1-\gamma) \mu^{(k)} + \gamma s , \quad s = \arg\max_{\nu\in D} \int  F'(\mu^{(k)})(x) d\nu(x),
\end{align}
where $F'$ is the functional derivative of $F$ with respect to $\mu$~\cite{santambrogio2017euclidean}.
It is easy to check that $s$ is always a Dirac measure at $\max_x F'(\mu^{(k)})(x)$. Hence,  $\mu^{(n-1)}$ is a sparse measure over $n$ particles as long as $\mu^{(0)} = \delta_{w_0}$. The compactness of $D$, convexity and smoothness of $F$ ensures the rate $O(1/n)$ for the convergence of Frank-Wolfe method~\cite{jaggi2013revisiting}.   
% \subsection{Proof of Lemma~\ref{lemma:suboptimality} }
% \begin{align}
%     F(\mu) - F(\mu_*) & \leq  F(\mu) \pm F(\widehat{\mu}) \pm F(\mu_*^{(n)}) - F(\mu_*) \label{eq:plus_minus}
% \end{align}
% According to the definition, we get $F(\widehat{\mu})-F(\mu_*^{(n)}) \leq 0$ which concludes the proof.
% \subsection*{Applications in machine learning}
% Consider minimizing the following energy distance 
% \begin{align}
%   \min_{\mu} \left(   E(\mu,\nu) = \int \| w- v \| \mu(dw) \mu(dv) - 2  \int \| w- v \| \mu(dw) \nu(dv) +  \int \| w- v \| \nu(dw) \nu(dv) \right)
% \end{align}
% Interestingly the above function is displacement convex but not strongly displacement convex. We claim that the above function relates to learning Fourier features. Francis Bach has remarked that the energy distance be decomposed as 
% \begin{align}
    
% \end{align}
\subsection{Proof of Lemma~\ref{lemma:energy_distance}}
The proof is a straightforward application of the key observation in \cite{hadi22}. \citet{hadi22} show the energy distance can be written alternatively as an MMD$_K$ distance with a positive definite kernel $K$, which is quadratic convex function in $\mu$. Since the kernel $K$ is Lipschitz, $L$ is smooth in the measure.   
\section{Applications for neural networks}
\subsection{Proof of Corollary~\ref{cor:neural_nets}}
\cite{hadi22} proves that $L$ is equivalent to the $E$ in polar coordinates. Invoking the part b of Theorem~\ref{thm:nonsmooth} concludes the rate.
